# Supplementary material for: Multicast Transmission Design with Enhanced DoF for MIMO Coded Caching Systems
Source: arXiv:2304.13827 source file (2023-11-23)
Supplement: Supplementary file 1 [file Appendix.tex]

 %\begin{center}




% \subsection{\textbf{Algorithm 1}}
%  \label{F}
%   \begin{algorithm}[t]
% 	\caption{SCA of \eqref{eq:P_optimum2} }
% 		\begin{enumerate}
% 		\item \textbf{Initialize} 
% 		$\bar{\BK}_{\tilde{\Bx}_{\CT^{}}}, \CT \in {\CS}_k^{\CK}, \forall k \in \CK$, and $Er_\text{SCA} = 10^{-4} $. 
% 		\item \textbf{Repeat} 
% 		\item Solve convex problem (\refeq{eq:P_optimum2}) for given $\bar{\BK}_{\tilde{\Bx}_{\CT^{}}}$ to 
% 		obtain ${\BK}_{\tilde{\Bx}_{\CT^{}}},  \CT \in {\CS}_k^{\CK}, \forall k \in \CK$ and $R$. 
% 		\item update $\bar{\BK}_{\tilde{\Bx}_{\CT^{}}}  = {\BK}_{\tilde{\Bx}_{\CT^{}}},  \CT \in {\CS}_k^{\CK}, \forall k \in \CK$.
% 		\item \textbf{Untill}  
% 		${\Big|R - 
% 		\Bar{R}\Big|}$ $\leq$ 
% 		$Er_\text{SCA}$
% 		\item \textbf{Output} ${\BK}_{\tilde{\Bx}_{\CT^{}}}^* = 
% 		\bar{\BK}_{\tilde{\Bx}_{\CT^{}}},  \CT \in {\CS}_k^{\CK}, \forall k \in \CK$   
% 	\end{enumerate}
% \end{algorithm}
% \subsection{Special case of general transmission vector}
%   \label{A}
% A special case of (\refeq{eq:Psig}) is a linear transmit precoding, where the transmit vector is expressed as~\cite{tolli2018multicast}:   
%  \begin{IEEEeqnarray}{lll}\label{eq:Linear Precoder}
% 		{\Bx}(1)= (A_2\oplus B_1)\Bw_{1,2} + (A_3\oplus C_1)\Bw_{1,3} + (B_3\oplus C_2) \Bw_{2,3} ,\nonumber\\
% 	\end{IEEEeqnarray}
% In (\refeq{eq:Linear Precoder}) $ \Bw_{\mathcal{T}}$ denotes multicast beamformer, $\mathcal{T} \in \{\{1,2\}, \{1,3\}, \{2,3\}\}$.
    
  %\end{center}


%\begin{center}
    %{\bf APPENDIX \Romannum{2}}.
%     \subsection{Symmetric rate optimization for $ L = 4 , G = 2 $ and $\eta > 1$} 
%   \label{B}
%  The symmetric rate maximization for $\CK = \{1,2,3\}$ with $\Omega = 3$ is expressed as 
% \begin{equation}
% \label{eq:P_optimum1_K3}
% \begin{aligned}
% &\max_{\mathbf{K}_{{\mathbf{x}}_{\mathcal{T}}}, R}  
%   R \\
%     &s.t.\quad R \leq \log|\mathbf{I}+\mathbf{H}_1 \mathbf{K}_{{\Bx}_{1,2}}\mathbf{H}_1^H\BQ_{1}^{-1}|, \; \\
%     &\quad\:\quad R  \leq \log|\mathbf{I}+\mathbf{H}_1 \mathbf{K}_{{\Bx}_{1,3}}\mathbf{H}_1^H\BQ_{1}^{-1}|, \; \\
%     & \quad\:\quad  R \leq \frac{1}{2}\log|\mathbf{I}+\mathbf{H}_1 (\mathbf{K}_{{\Bx}_{1,2} } + \mathbf{K}_{{\Bx}_{1,3} })\mathbf{H}_1^H\BQ_{1}^{-1}|,\: \\
%     &\quad\:\quad R  \leq \log|\mathbf{I}+\mathbf{H}_2 \mathbf{K}_{{\Bx}_{1,2}}\mathbf{H}_2^H\BQ_{2}^{-1}|, \; \\
%     & \quad\:\quad R  \leq \log|\mathbf{I}+\mathbf{H}_2 \mathbf{K}_{{\Bx}_{1,3}}\mathbf{H}_2^H\BQ_{2}^{-1}|, \; \\
%     & \quad\:\quad R  \leq \frac{1}{2}\log|\mathbf{I}+\mathbf{H}_2 (\mathbf{K}_{{\Bx}_{1,2} } + \mathbf{K}_{{\Bx}_{2,3} })\mathbf{H}_2^H\BQ_{2}^{-1}|,\: \\
%     &\quad\:\quad R \leq \log|\mathbf{I}+\mathbf{H}_3 \mathbf{K}_{{\Bx}_{1,3}}\mathbf{H}_3^H\BQ_{3}^{-1}|, \; \\
%     & \quad\:\quad R \leq \log|\mathbf{I}+\mathbf{H}_3 \mathbf{K}_{{\Bx}_{2,3}}\mathbf{H}_3^H\BQ_{3}^{-1}|, \; \\
%     & \quad\:\quad R  \leq \frac{1}{2}\log|\mathbf{I}+\mathbf{H}_3 (\mathbf{K}_{{\Bx}_{1,3} } + \mathbf{K}_{{\Bx}_{2,3} })\mathbf{H}_3^H\BQ_{3}^{-1}|, \; \\
%     & \quad\:\quad \sum_{\mathcal{T} \in \{\{1,2\}, \{1,3\}, \{2,3\}\} }\text{Tr}(\mathbf{K}_{{\Bx}_{\mathcal{T}}})
% 	  \leq P_T
% \end{aligned}
% \end{equation}

% where $\BQ_{1}  =  N_0\mathbf{I}+\mathbf{H}_1 \mathbf{K}_{{\Bx}_{2,3}}\mathbf{H}_1^H $, $\BQ_{2}  =   N_0 \mathbf{I}+\mathbf{H}_2 \mathbf{K}_{{\Bx}_{1,3}}\mathbf{H}_2^H $, and $\BQ_{3}  =   N_0\mathbf{I}+\mathbf{H}_3 \mathbf{K}_{{\Bx}_{1,2}}\mathbf{H}_3^H $. 

% Problem (\refeq{eq:P_optimum1_K3}) is nonconvex; however, it is readily solved by the proposed SCA in \textbf{Algorithm 1}. 
    % \subsection{Symmetric rate optimization for $L = G = 2$ and $\eta = 1$}

%{\bf APPENDIX \Romannum{3}}
%   \label{C}

%     Given the multicast signal vector ${\Bx}= {\Bx}_{1,2,3}$, and $ \{\Omega  = 3,t = 2 \}$, the received signal vector is 
% \begin{IEEEeqnarray}{lll}\label{eq:rx_sigsymm}
%   \By_1 = \BH_1 {\Bx}_{1, 2, 3} + \Bz_1\; ,\nonumber\\
%   \By_2 = \BH_2  {\Bx}_{1, 2, 3} + \Bz_2\; ,\nonumber\\
%   \By_3 = \BH_3  {\Bx}_{1, 2, 3} +  \Bz_3\;\nonumber ,
% \end{IEEEeqnarray}
% in which there is no interference and the optimal solution is obtained by
% \begin{equation}
% \label{eq:P_optimum1_K1_symexm}
% \begin{aligned}
% &\max_{\mathbf{K}_{{\Bx}_{1, 2, 3}}, R_{}^k} \min_{k\in \CK} 
%   (R_{}^1, R_{}^2, R_{}^3) \\
%     &s.t.\quad R_{}^{1} \leq \log|\mathbf{I}+\mathbf{H}_1 \mathbf{K}_{{\Bx}_{1, 2, 3}}\mathbf{H}_1^H|, \; \\
%     &\quad\:\quad R_{}^{2} \leq \log|\mathbf{I}+\mathbf{H}_2 \mathbf{K}_{{\Bx}_{1, 2, 3}}\mathbf{H}_2^H|, \; \\
%     &\quad\:\quad R_{}^{3} \leq \log|\mathbf{I}+\mathbf{H}_3 \mathbf{K}_{{\Bx}_{1, 2, 3}}\mathbf{H}_3^H|, \; \\
%     & \quad\:\quad \text{Tr}(\mathbf{K}_{{\Bx}_{1, 2, 3}})
% 	  \leq P_T
% \end{aligned}
% \end{equation}
% where \eqref{eq:P_optimum1_K1_symexm} could be efficiently tackled with CVX solvers. Following the same procedures as in the previous examples, we have $R_{sym} = \frac{10 {\binom{10}{2}}}{{\sum_i^{120}{\frac{1}{R_i}}}}$ 
% \begin{equation}
% \label{eq:symmetric_rate_ergodic_case1k51}
% R_{sym} =  \frac{10 {\binom{10}{2}}}{\binom{10}{5}}R_{erg}  \; ,
% \end{equation}

  %\end{center}

  

 % \appendix

% \chapter{\Romannum{1}}

% \chapter{B}
% \label{B}

% \chapter{third}
% \label{section:third}


% \subsection{Examples}
% \label{D}
% \subsection{Scenario 1: $L = 2$, $G = 2$ and $t=1$, $t = 2$} 
% \begin{exmp}
%     \label{exmp:x6serv}
% \normalfont

% In this example, given $L = 2$, $G = 2$, the number of served users can be $\Omega = \{2, 3, 4\}$, making requests for files from $\{A-B, A-C, A-D\}$, respectively, and the CC gain $t$ is either 1 or 2. % $t \in \{1, 2\}$. 
%  %In this scenario, the number of served users belong to set $\Omega = \{2, 3, 4\}$, each with CC gain $t \in \{1, 2\}$, each making requests for files from $\{A-B, A-C, A-D\}$, respectively. 
%  As a part of the content delivery process, users demand their required files. Then, the multicast transmission signal vectors for these setups are defined as: 
%  \[
% {\Bx}= \begin{cases}
%      {\Bx}_{1,2}   + {\Bx}_{1,3}  +{\Bx}_{2,3},& \text{if } \{\Omega  = 3 , t = 1 \},\\
%      {\Bx}_{1,2,3}   + {\Bx}_{1, 2, 4}  +{\Bx}_{1,3, 4} +{\Bx}_{2, 3, 4} , & \text{if } \{\Omega  = 4 ,t = 2 \}\\
%       {\Bx}_{1,2}, & \text{if } \{\Omega  = 2 , t = 1 \},\\
%       {\Bx}_{1,2,3},               & \text{if }  \{\Omega  = 3 ,t = 2 \},
% \end{cases}
% \]
% given the received signal at user $k$ is  
% \begin{IEEEeqnarray}{lll}\label{eq:rx_sigsym}
% 		\By_k = \BH_k {\Bx} +\Bz_k,\; 
% \end{IEEEeqnarray}
%  The first and second signal vectors coincide with a 2- and 3-dimensional MAC channel, respectively, and the symmetric rate is calculated in the same manner as in examples \ref{exmp:x3serv}, and \ref{exmp:x4serv} (except considering $t = 2$). The third and fourth cases, however, do not involve an equivalent MAC channel and are treated differently, as explained in Appendix \ref{C}. In fact, we need to work through all of these different parameter combinations to determine which setup achieves the maximum achievable DoF.
% \end{exmp}
% \begin{exmp}
%     \label{exmp:x7serv}
% \normalfont
%  We assume a similar setup to example~\ref{exmp:x3serv}; however, $L = 3$, which results in a non-divisible $\frac{L}{G}$. 
% Assuming that the number of served users is $\Omega = \{2, 3, 4\}$, we have the following signal vectors
%  \[
% {\Bx}= \begin{cases}
%      {\Bx}_{1,2}   + {\Bx}_{1,3} + {\Bx}_{1,4} +{\Bx}_{2,3} + {\Bx}_{2,4} +{\Bx}_{3,4},& \text{if } \{\Omega  = 4 \},\\
%      {\Bx}_{1,2}   + {\Bx}_{1,3}  +{\Bx}_{2,3}, & \text{if } \{\Omega  = 3\},\\
%      {\Bx}_{1,2}, & \text{if } \{\Omega  = 2 \}.
% \end{cases}
% \]
% In accordance with the previous examples of multicast transmission signals, one can compute the symmetric rate in the same way.
% \end{exmp}
% \subsection{Scenario 1: $L = 4$, $G = 2$, and $t=2$} 
% \begin{exmp}
%     \label{exmp:x8serv}
% \normalfont
 
%  Another example of $\eta > 1$ can be found here, in which $t = 2$  and the number of users served is set to $\Omega = \{4, 5\}$.
%   As a consequence, we have
%  \[
% {\Bx}=\begin{cases}
%      \tilde{\Bx}_{1,2,3}   + \tilde{\Bx}_{1, 2, 4} +  \tilde{\Bx}_{1, 2, 5} +\tilde{\Bx}_{1,3, 4} +\tilde{\Bx}_{1,3, 5}  \\  + \tilde{\Bx}_{1,4, 5} + \tilde{\Bx}_{2, 3, 4} + \tilde{\Bx}_{2, 3, 5} + \tilde{\Bx}_{2, 4, 5} + \tilde{\Bx}_{3, 4, 5},& \text{if } \{\Omega  = 5 \},\\
%       \tilde{\Bx}_{1,2,3}   + \tilde{\Bx}_{1, 2, 4}  +\tilde{\Bx}_{1,3, 4} +\tilde{\Bx}_{2, 3, 4}, & \text{if } \{\Omega  = 4 \}
% \end{cases}
% \]
% \end{exmp}
